# Supplementary material for: Tragedy Plus Time: Capturing Unintended Human Activities from Weakly-labeled Videos
Source: arXiv:2204.13548 source file (2022-04-28)
Supplement: Supplementary file 4 [file quant-results_appendix_copy_compressed.pdf]

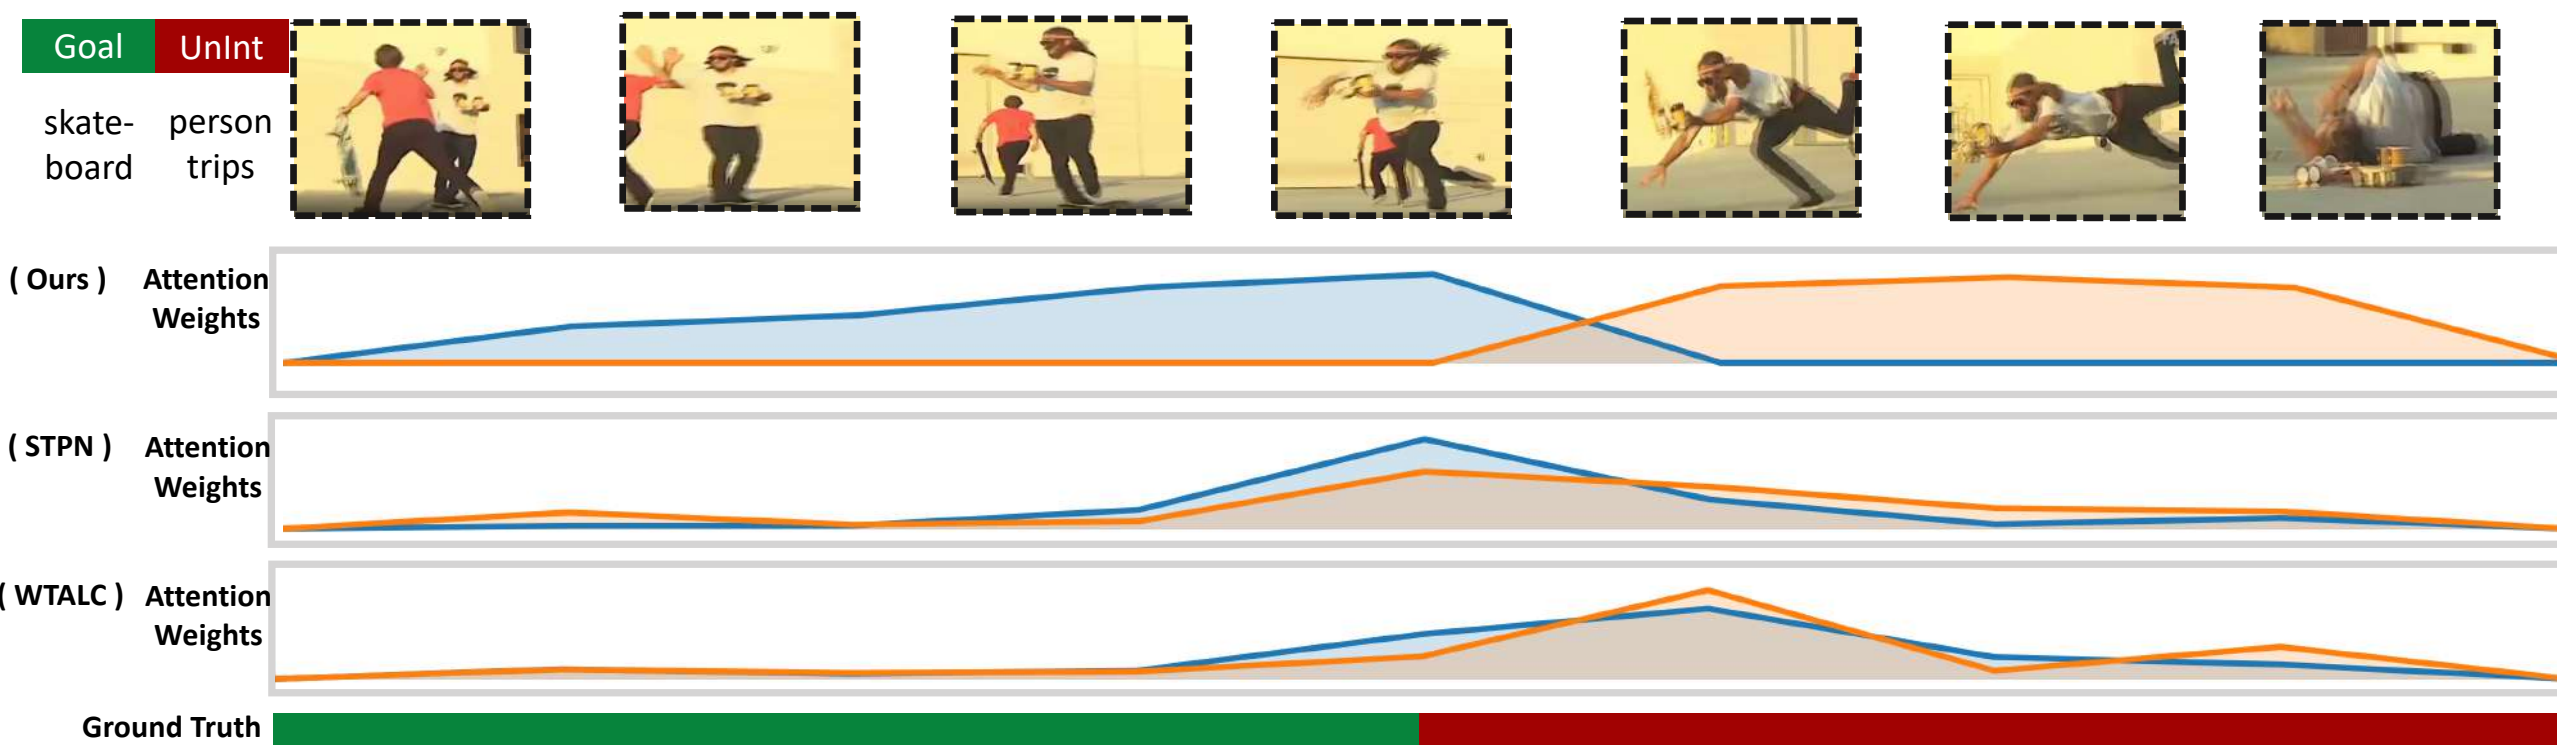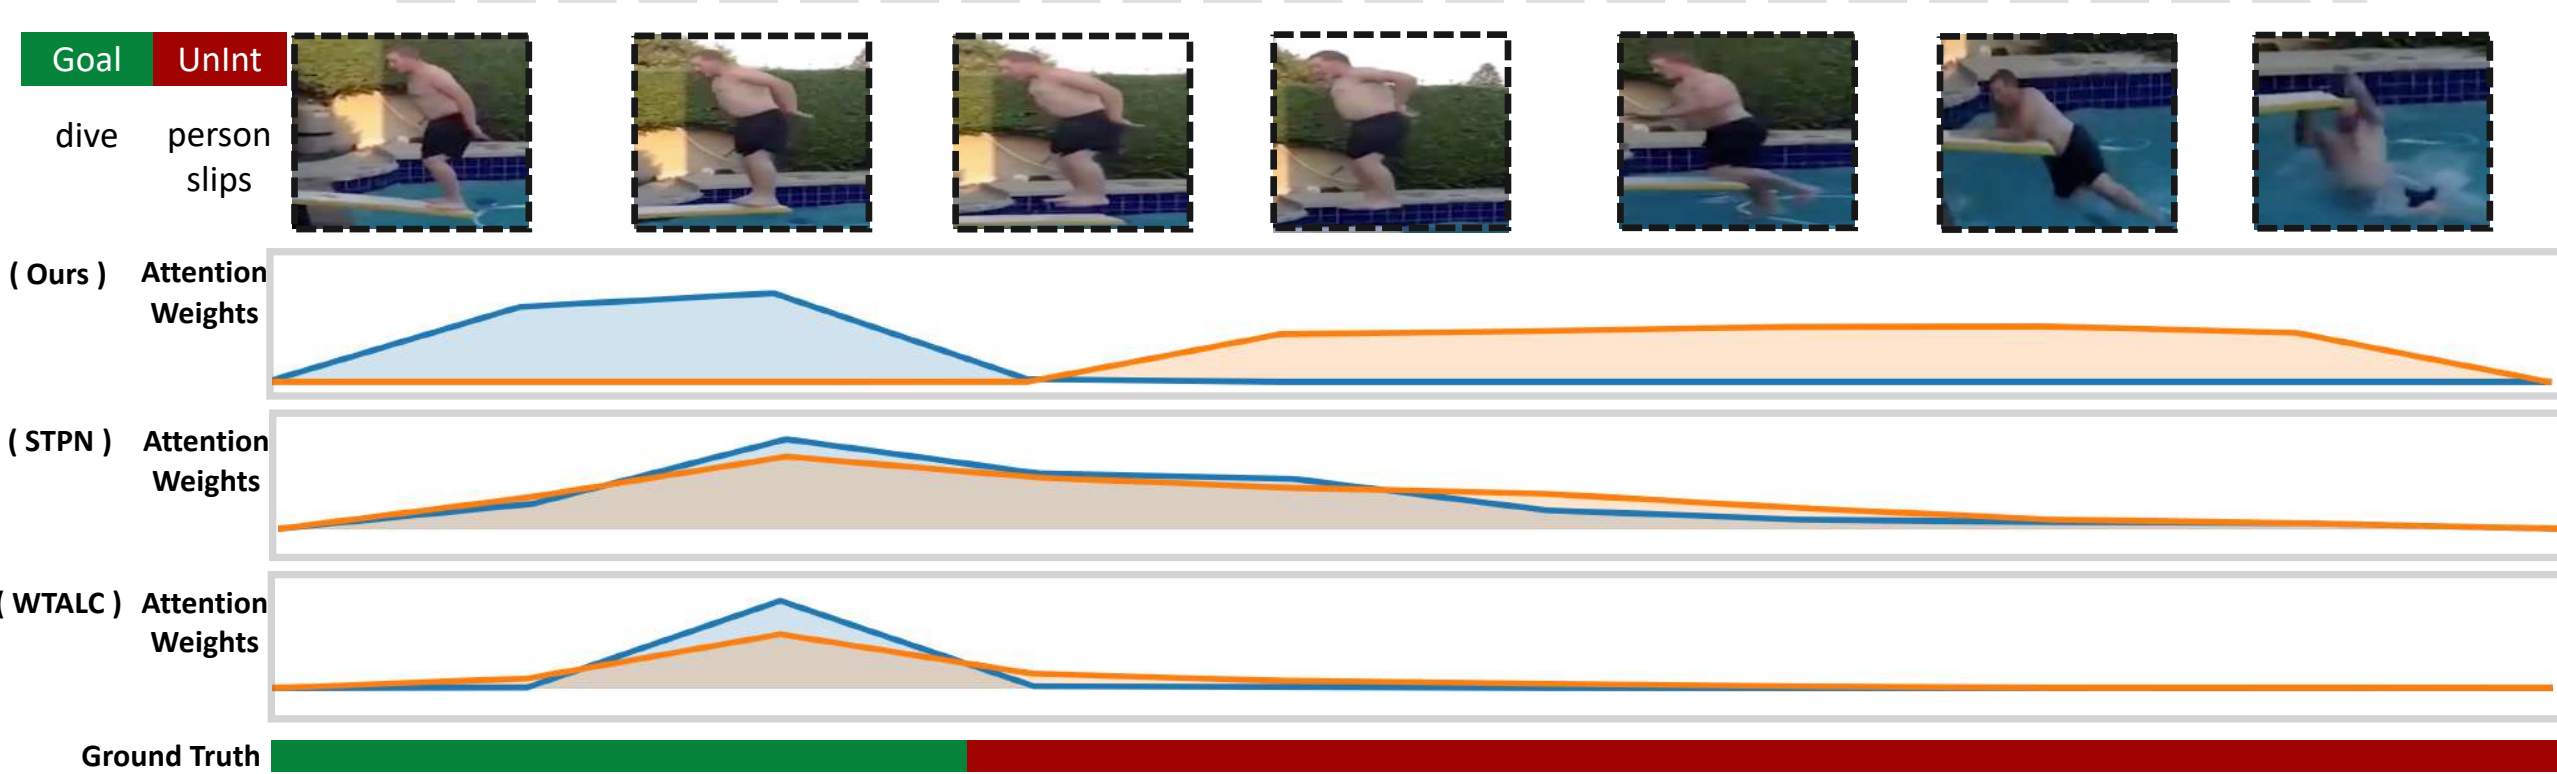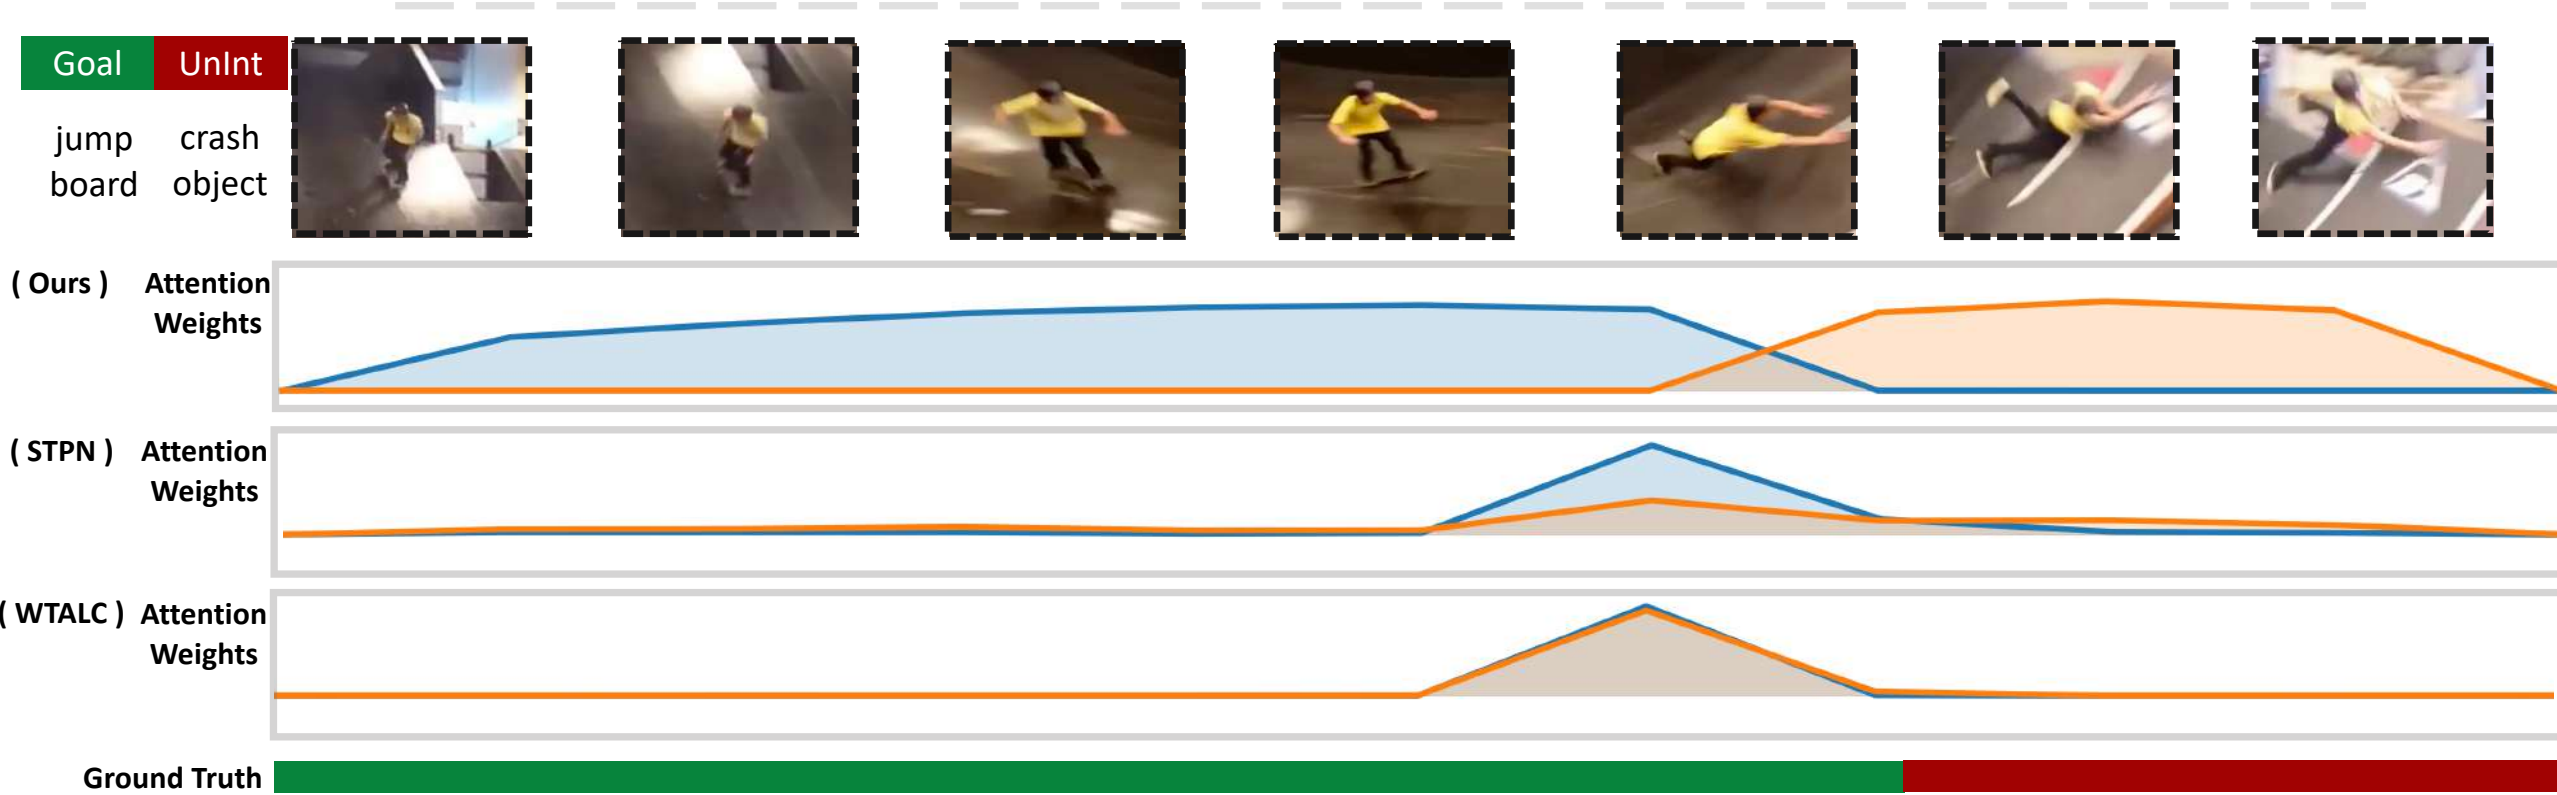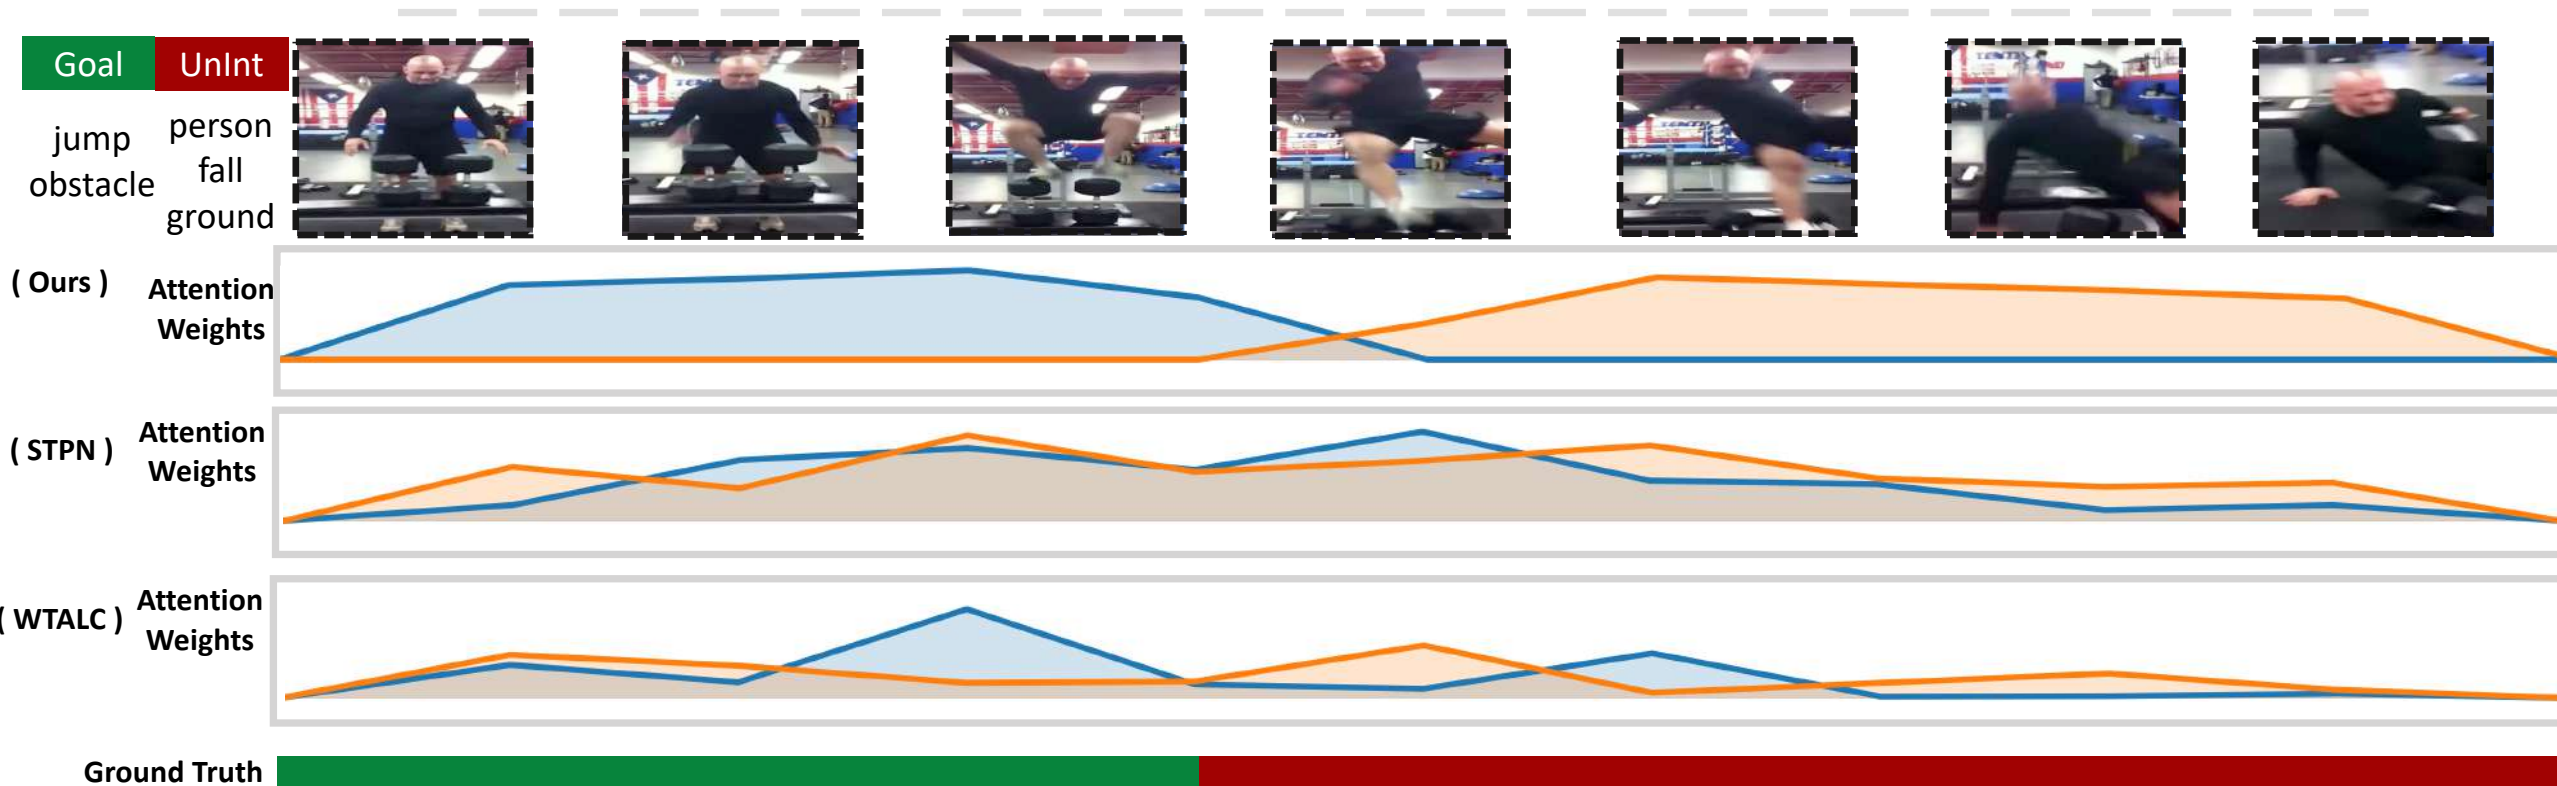

|                                                                                                           |                                                                                                                       |
|-----------------------------------------------------------------------------------------------------------|-----------------------------------------------------------------------------------------------------------------------|
| 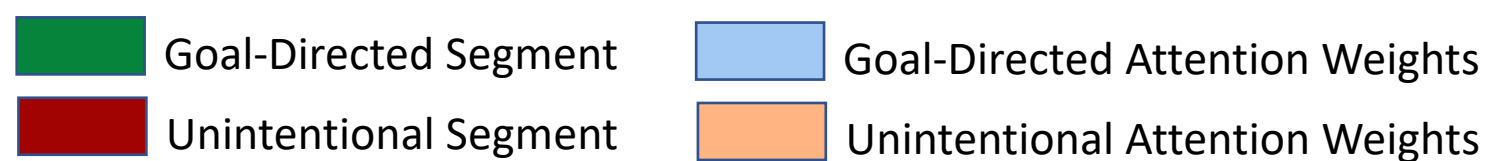 Goal-Directed Segment | 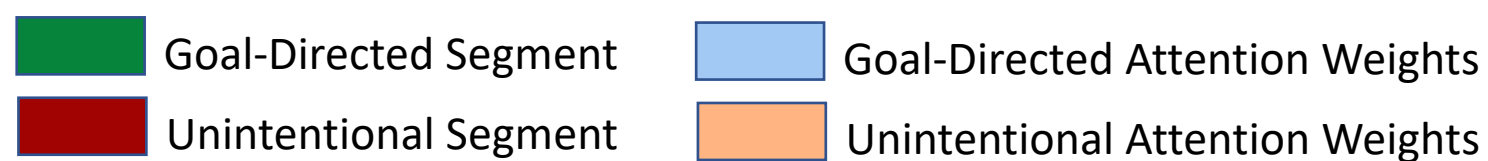 Goal-Directed Attention Weights |
| 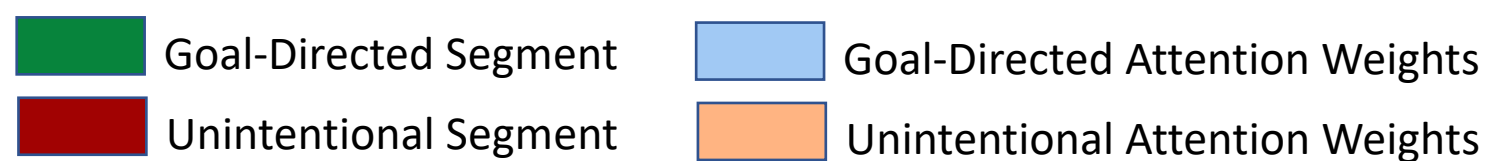 Unintentional Segment | 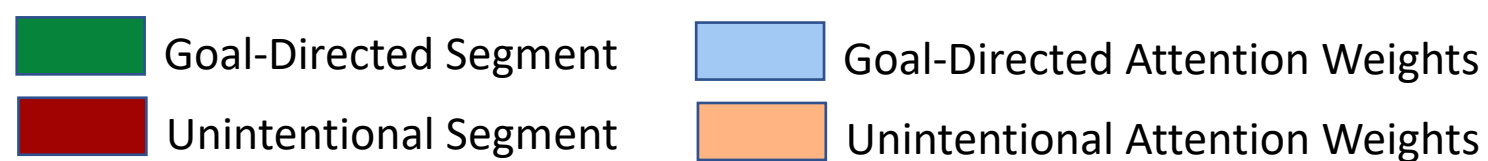 Unintentional Attention Weights |



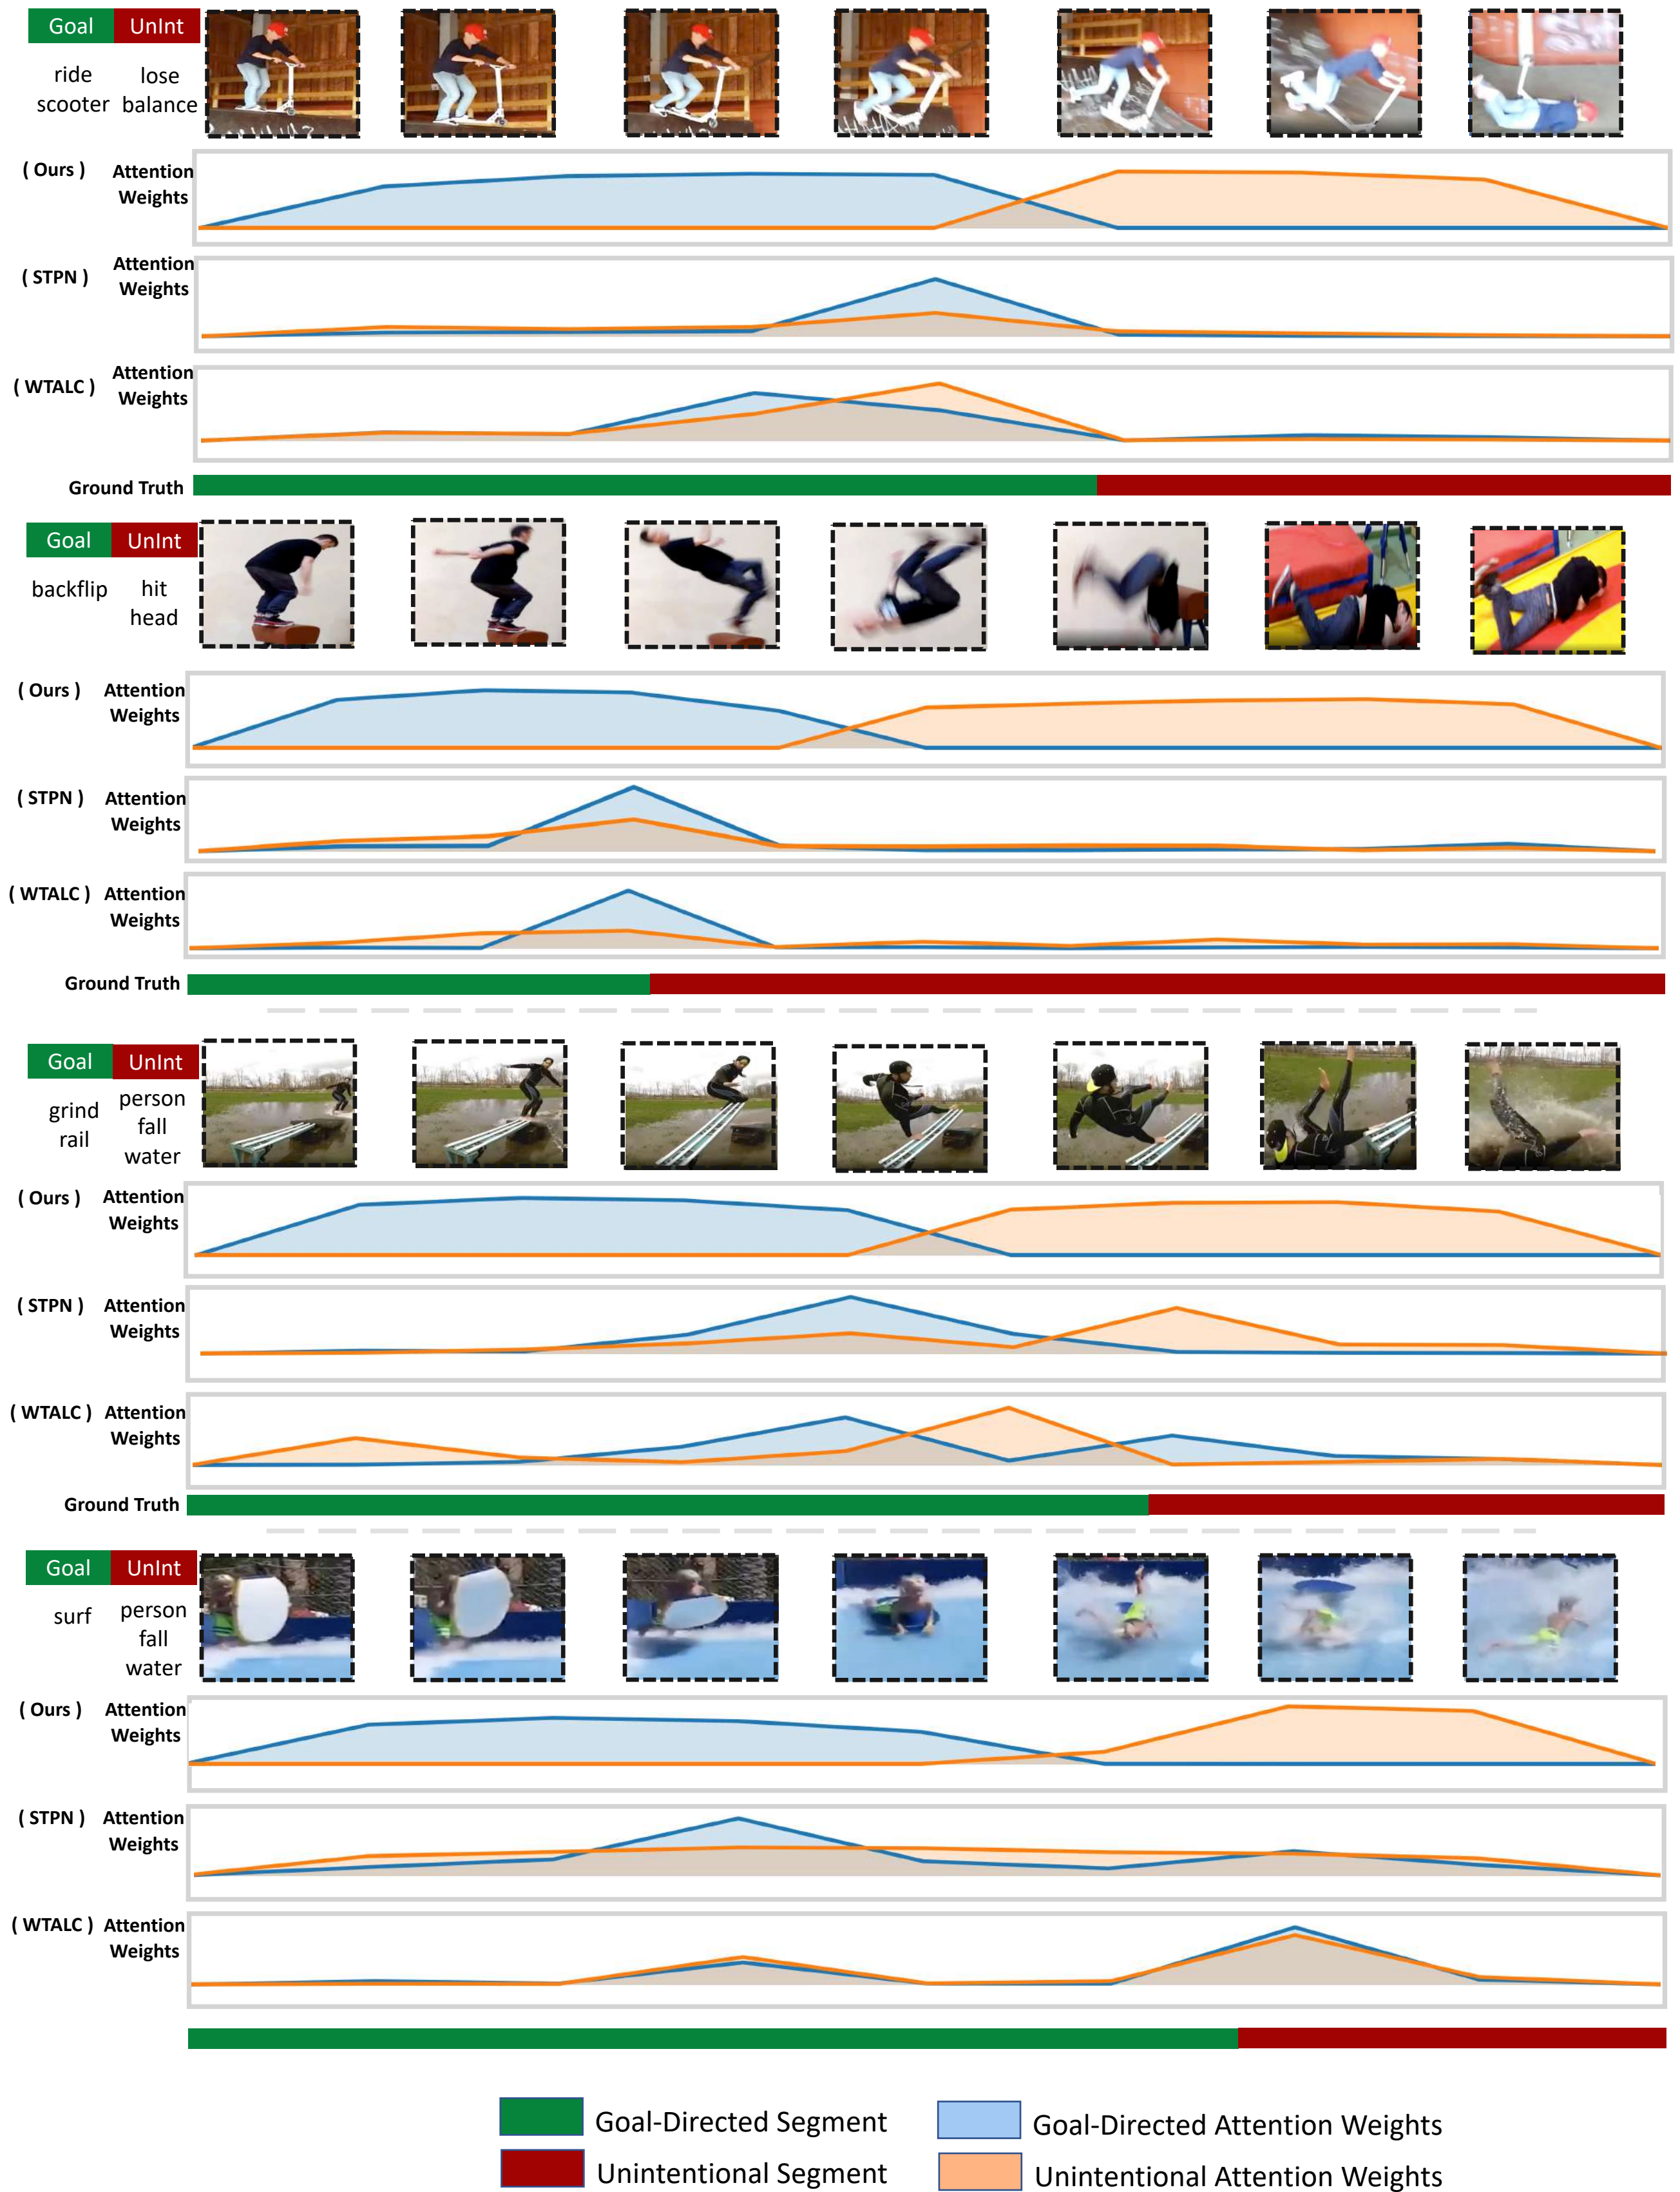



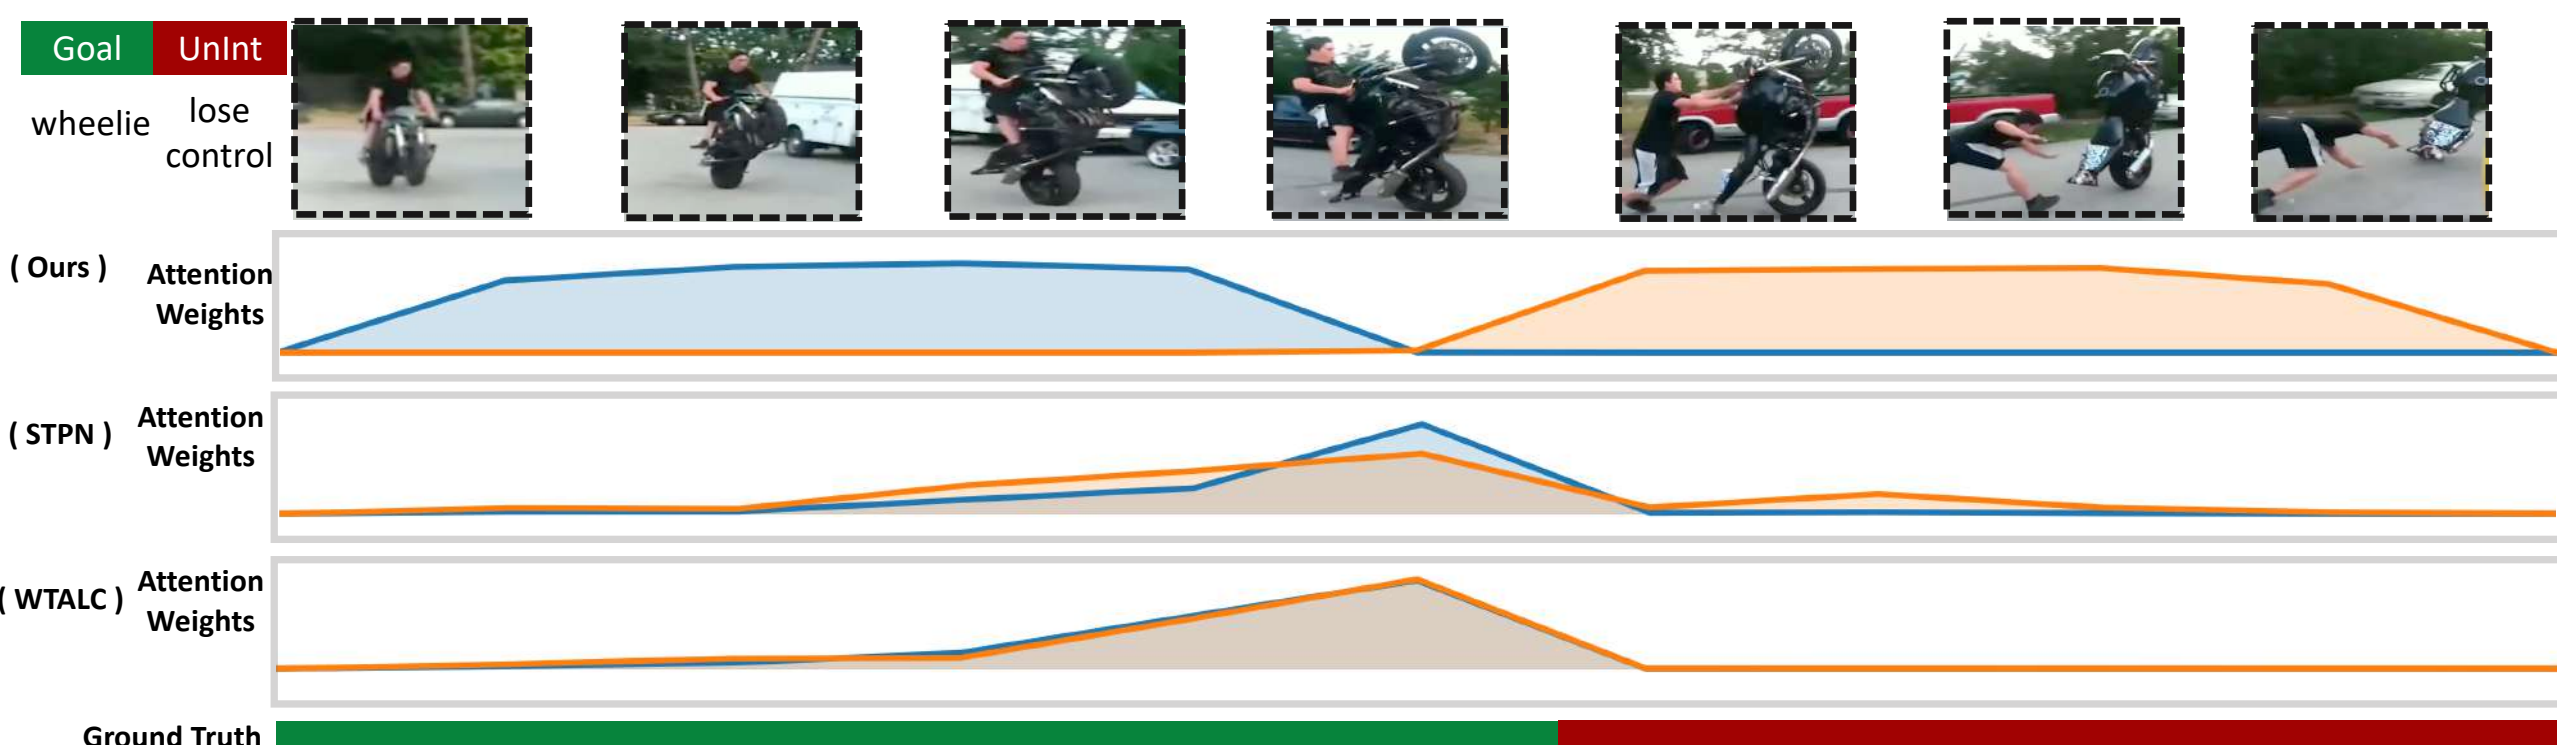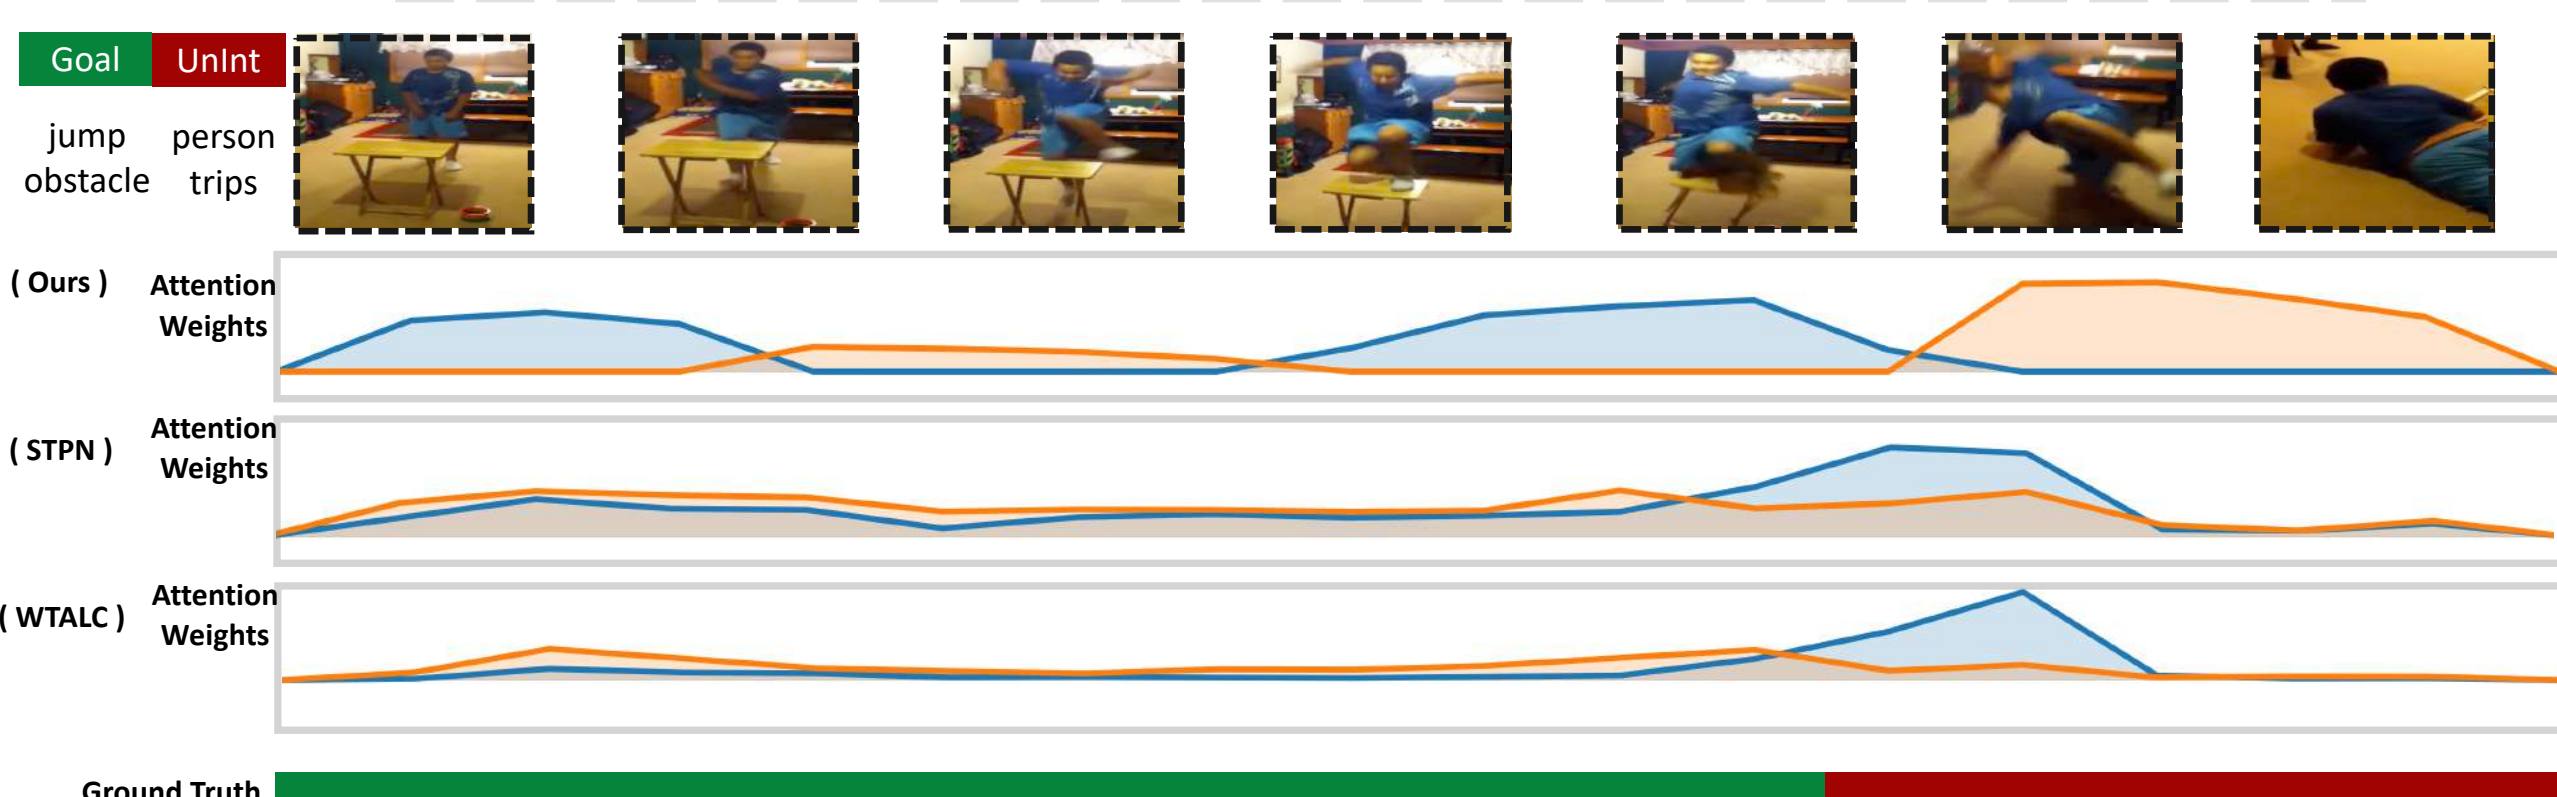

Goal-Directed Segment

Unintentional Segment
